# Supplementary material for: Structure from Action: Learning Interactions for Articulated Object 3D Structure Discovery
Source: arXiv:2207.08997 source file (2023-04-07)
Supplement: Supplementary file 1 [file supp.tex]

\newpage
\appendix

% The document below is the supplementary material submitted during the paper submission phase, and we attached it here for easy access. 

\section{Simulation Environment}

\label{sec:appx-sim}
We use the PyBullet physics simulator \cite{coumans2016pybullet} for generating the training data and evaluating the SfA pipeline (referred to on L593). Five depth cameras with known positions and camera parameters are placed around the object: one at the top with a birds-eye-view, and one on each of the four sides of the object. The observation is generated by fusing the back-projected depth maps from each of the cameras. When an object is loaded, the object will be resized to fit in a $2^3$ cube. The scaling factor, initial position, and orientation are all randomly sampled from a normal distribution during training and testing. The state of each joint is randomized each time the object is loaded into the simulator. 

\label{sec:real-world-supp}
\section{Real World Experimental Setup}
We utilize two main methods to capture real-world point cloud data to test and validate the SfA pipeline. (referred to on L590-591) Method one: we mounted a RealSense RGBD camera on the wrist of a UR5 robot manipulator. Once we place an object on the table, we move the camera to five preset poses, capturing the RGBD frames. Finally, we combine the posed partial point clouds from the RGBD frames into one single point cloud for the SfA pipeline. After action inference, we manually manipulate the part of the object based on the inferred action. We repeat this process for four steps. Method two: we take advantage of the LiDAR sensor found on smartphones (iPhone 14 Pro) to capture the complete point cloud of the object. Similar to the RealSense capture system, after the action inference step, we manually move the part of the object based on the inferred action. We repeat this process for four steps. 

\section{Ground Truth Generation}

\label{sec:appx-gt-action}
\textbf{Action Supervision from Motion.} In Sec. 3.2, we describe using the observed 3D scene flow as the supervision signal for the interaction module. To generate the supervision, we load the training objects from the PartNet-Mobility dataset \cite{Xiang_2020} in the PyBullet physics simulator \cite{coumans2016pybullet}. We allow the ground truth generation algorithm to interact with each training object $N=5$ times, since all objects in the dataset have five parts or fewer. At each timestep, we use the joint parameters specified in the object URDF file to randomly generate a new target joint state for a single non-fixed joint in the object. Then, we change that joint state by at least 1/4 of the joint's range of motion to arrive at a new target joint state. By changing the joint state, we have effectively moved one part of the object. We capture observations before and after the part movement and use the ground truth correspondence provided by the simulation environment to generate the forward 3D scene flow, only during training. Within $N$ steps, the algorithm will move each part at least once by altering the joint states, exposing the full kinematic structure of the object. Given new URDF files of other object categories and objects with novel kinematic structures, this method of ground truth generation is easily cheap to execute and scaleable. 

\label{sec:appx-gt-parts}
\textbf{Persistent Part Aggregation.} We use the same method described above to generate the ground truth parts labels used to train the persistent part aggregation module described in Sec. 3.3. 
At the initial timestep, before a joint state has changed, part label 1 is given to all points on the object, as no part has been discovered yet. Once a joint state has changed, a new part has been discovered. This newly discovered part will be assigned a new part label 2, while the rest of the object will keep the part label 1. In the following steps, all undiscovered parts will be moved at least once, and they will each receive a unique integer part label. In the case of movement of a discovered part, the part and the rest of the object will maintain their parts labels. 

Initially, the unobserved occluded surfaces in the object is not included in the ground truth parts segmentation. As more surfaces and parts of the objects are observed by the five-camera array, the new observations are aggregated with the most up-to-date parts segmentation, building up a more and more complete representation of the object parts geometry. If an already seen part of the object becomes occluded after some interaction, the parts segmentation will maintain the part integrity, thus encouraging the parts aggregation model to learn parts permanence.

\section{Network Architecture}
\label{sec:appx-action-net}
\textbf{Action Network.} The action network is trained using the SGD optimizer with an initial learning rate of 0.5 over 50 epochs, and a multi-step learning rate scheduler. All hyperparameters are selected based on the original Point Transformer \cite{Zhao2020} implementation. Both the hold prediction and push prediction networks have 4 blocks, 256 transformer dimensions, progressive downsampling by 4x, and consider 16 points for nearest neighbors. We use farthest point sampling to downsample the observation point cloud to 2048 points. 

\label{sec:appx-parts-net}
\textbf{Part Aggregation Network.} The parts aggregation network is trained using the Adam optimizer with 2e-4 learning rate, batch size 9, over 20 epochs. The network follows the 3D UNet \cite{Ronneberger2015} architecture with residual connections similar to those proposed by \cite{He2016}. The input of the network is: the voxelized observation at time $t$ before the interaction, the voxelized parts segmentation at time $t$, and the voxelized observation after the interaction at $t+1$. The output of the network is a voxel volume with each voxel representing the parts label using 1-hot encoding. The network is comprised of an encoder and decoder sub-network. The encoder network has 8 residual blocks, each block consists of 2 3D convolutional layers with kernel size $3 \times 3 \times 3$, batch normal layers, and leaky ReLU activation layers. The decoder network consists of 4 ResNet 3D upsampling blocks. Within each block, there is one trilinear upsampling layer followed by a convolutional layer and 2 ResNet blocks. After the last ResNet 3D upsampling block, we apply another 3D convolution layer with $1 \times 1 \times 1$ kernel size and channel dimension 8, which is the final output channel dimension. There are skip connections between the decoder and encoder network, based on the original UNet \cite{Ronneberger2015} architecture. 

\label{sec:appx-joints-net}
\textbf{Joints Network.} The joint network is trained using the Adam optimizer with 5e-4 learning rate over 20 epochs. The network architecture is nearly identical to the parts aggregation network. The two major differences are: 1) joints network only considers the before and after observation, without the previous history, 2) the joints network has 8 channels that represent the joint parameters. The joint network and the part aggregation network are trained separately. 

\section{Details on Joint Inference Algorithm}
\label{sec:appx-joints}
In Sec. 3.4, we present the joint inference model which predicts the joint parameters of one single joint that connects the most recently moved part to the rest of the object. During multiple interaction steps, we aggregate the joint parameters of many different joints using the following method. The key idea is to build a dictionary containing part's segmentation label to joint parameter pairs. At each interaction step, assuming one part has been moved, the part aggregation model returns the moved part segmentation label $id_{moved}$. The joints model returns the joint parameters, $J_{type}, \;\; J_{axis}, \;\; J_{position}$ denoting the joint type, axis, and position, associated with $id_{moved}$. Given this information, we add the key-value pair $id_{moved}: \{J_{type}, \;\; J_{axis}, \;\; J_{position}\}$ to our dictionary. If a part is moved more than once, we maintain a collection of $\{J_{type}, \;\; J_{axis}, \;\; J_{position}\}$. The final joint parameters will be the median of all inferred values. After all interaction steps, we use all key-value pairs in the dictionary to generate the 3D articulated CAD model (i.e. the URDF file). 

\section{Constructing an Articulated CAD Model}
\label{sec:appx-reconstruction}

Given the part volume, we can generate the 3D part mesh of each part. Then, combined with the joint parameters, we generate a consolidated URDF file describing the articulated 3D CAD model. (referred to on L537-539) We treat the inverted probability volume for each segmented part $\hat{\mathcal{H}_t} = 1 - \mathcal{H}_t$ similar to a truncated distance function, where 0 indicates the surface, and the value at each cell represents the truncated distance to that 3D surface.
We then apply marching cubes to extract the zero-crossing surface. 
Once we have the 3D part mesh for each part, we save them to disk as \texttt{.obj} files. We first create all \texttt{<link>} tags using the \texttt{.obj} files. Then, by using the part number to joint parameter key-value pairs, we create the full URDF file by adding in the \texttt{<joint>} tags. We assume that each part is connected to the baselink, which is designated as part 1. 

\section{Heuristics Joint Estimation Baseline }
\label{sec:appx-joints-baseline}
To validate our learned joint estimation module, we developed a heuristic-based joint parameter estimation algorithm using the parts segmentation masks predicted by the parts aggregation model. (referred to on L689-690) The key idea is to obtain two point clouds of only the moved part before and after the interaction. By using ICP, we can estimate a SE(3) transform of the part movement. By using some heuristics, we can determine based on the SE(3) transform, the joint type, joint axis, and joint position. To compute the two point clouds of the moved part, we exploit the segmentation mask of the moved part before and after the interaction. 

\section{Dataset}
\label{sec:appx-dataset}
We use the articulated objects provided by the PartNet-Mobility \cite{Xiang_2020} dataset. There are  48 unseen instances from 10 training categories listed in Tab 1 and 77 instances from 7 testing categories listed in Tab 2. To minimize simulation errors, we sampled from all available training instances to ensure the included instances will behave as expected in the PyBullet \cite{coumans2016pybullet} simulator.  We sample the storage furniture category more than other categories to achieve a good balance of revolute joints and prismatic joints and also objects with more than 2 parts. Additionally, we excluded any instances from the original PartNet-Mobility data with missing meshes or unstable simulation results. 

\clearpage

\begin{table*}[]
{
\centering
\setlength\tabcolsep{ 2.2 pt}
\vspace{-3mm}
\begin{tabular}{l|cccccccccc}
\toprule
     &\multicolumn{10}{c}{Training Categories }  \\ 
     &  
      \includegraphics[width = 0.035\linewidth]{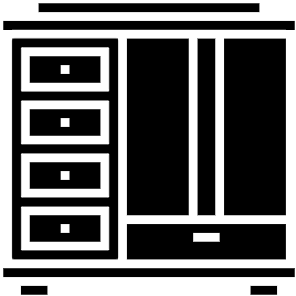} &
      \includegraphics[width = 0.035\linewidth]{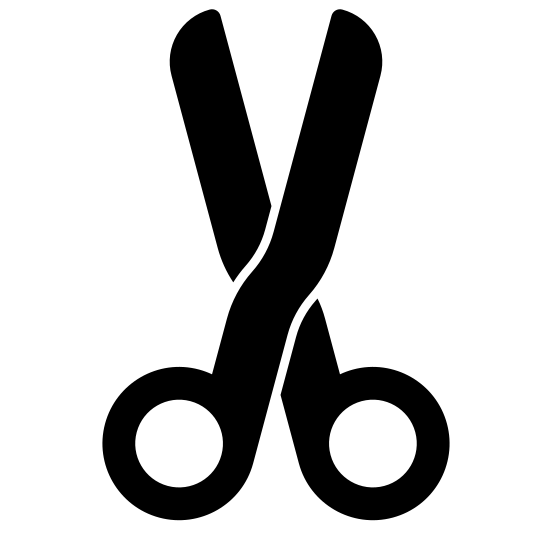} &
      \includegraphics[width = 0.035\linewidth]{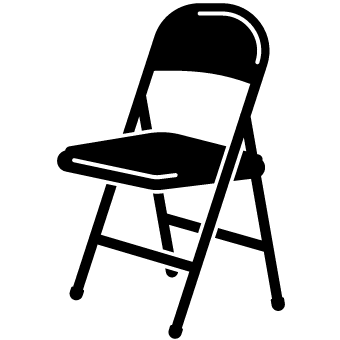} &
      \includegraphics[width = 0.035\linewidth]{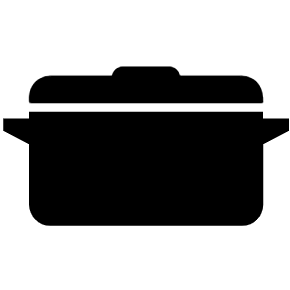} &
       \includegraphics[width = 0.035\linewidth]{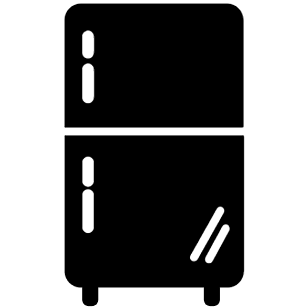} &
      \includegraphics[width = 0.035\linewidth]{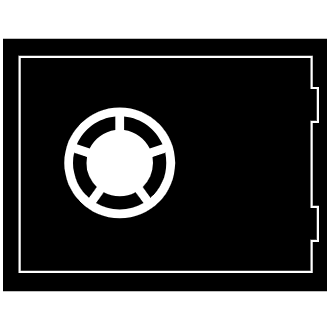} &
      \includegraphics[width = 0.035\linewidth]{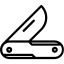} &
      \includegraphics[width = 0.035\linewidth]{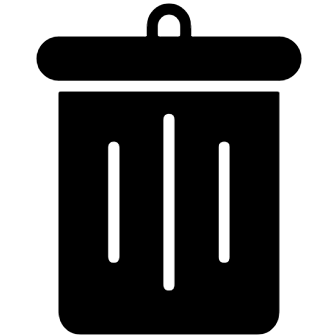} &
      \includegraphics[width = 0.035\linewidth]{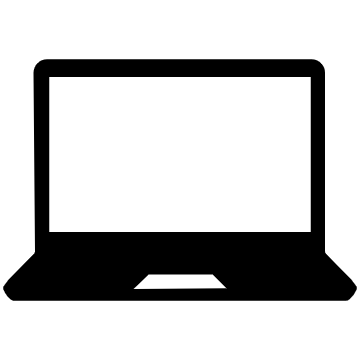} &
      \includegraphics[width = 0.035\linewidth]{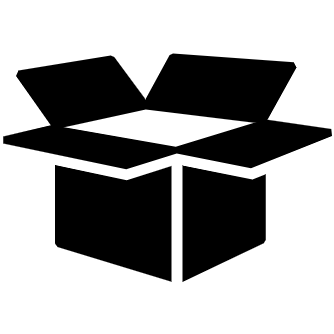} 
      \vspace{-0.2mm}
     \\
Category Name & Storage Furniture & Scissor & Folding Chair & Kitchen Pot & Refrigerator & Safe & Knife & Trashcan & Laptop & Box \\
\midrule
\end{tabular}
\caption{Training category icon names.}
}
\end{table*}

\begin{table*}[]
{ 
\centering
\setlength\tabcolsep{ 2.2 pt}
\vspace{-3mm}
\begin{tabular}{l|ccccccc}
\toprule
      & \multicolumn{7}{c}{Testing Categories}  \\ 
      & \includegraphics[width = 0.035\linewidth]{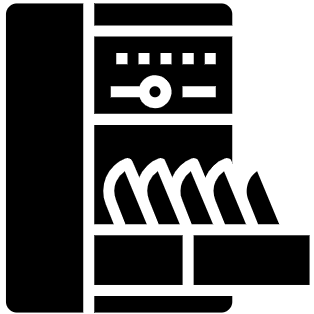} &
      \includegraphics[width = 0.035\linewidth]{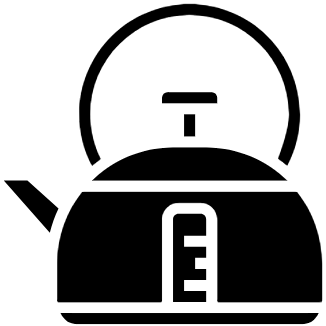}  &
      \includegraphics[width = 0.035\linewidth]{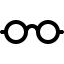} &
       \includegraphics[width = 0.035\linewidth]{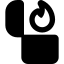} &
      \includegraphics[width = 0.035\linewidth]{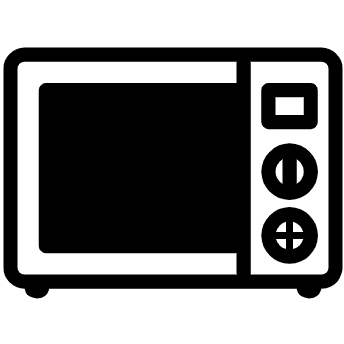} &
      \includegraphics[width = 0.035\linewidth]{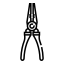} &
      \includegraphics[width = 0.035\linewidth]{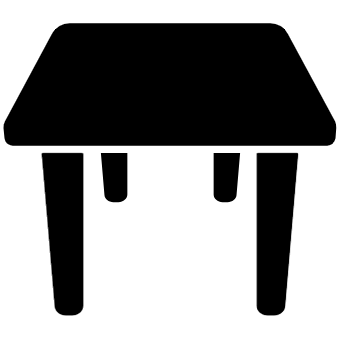}
      \vspace{-0.2mm}
     \\
Category Name & Dishwasher & Kettle & Eyeglasses & Lighter & Microwave & Plier & Table \\
\midrule
\end{tabular}
\caption{Testing category icon names}
}
\end{table*}

\SetKwComment{Comment}{/* }{ */}
\RestyleAlgo{ruled}
\begin{algorithm*}
\setstretch{1.25}
\SetAlgoLined
\caption{Heuristic Based Joint Estimation Algorithm}\label{alg:two}
\KwData{$V_{t-1}$, $V_{t}$, $\mathcal{H}_{t-1}$}
\KwResult{$J_{type}, J_{axis}, J_{position}$}
$\mathcal{H}_{t} \gets \texttt{part\_model.forward}(\mathcal{H}_{t-1}, \;\; V_{t-1}, \;\; V_{t})$  \Comment*[r]{Running inference on the part aggregation model.} 
$\mathcal{H}'_{t-1} \gets \texttt{part\_model.forward}(\mathcal{H}_{t}, \;\; V_{t}, \;\; V_{t-1})$ \\
$id_{moved} \gets \texttt{max\_occurrence}( abs( \mathcal{H}'_{t-1} - \mathcal{H}'_{t}))$ \\
$\mathcal{P}_t \gets \textit{where } \mathcal{H}_{t} \textit{ is } id_{moved} $ \\
$\mathcal{P}_{t-1} \gets \textit{where } \mathcal{H}_{t-1} \textit{ is } id_{moved} $ \\
$T \gets \texttt{ICP}(P_t, \;\; \mathcal{P}_{t-1})$ \Comment*[r]{$T$ is a SE(3) transform} 
$\theta,\;\; \Vec{a} \gets \texttt{axis\_rotation}(T)$ \Comment*[r]{Finds the axis of rotation given a SE3 transform.} 
\eIf{$\theta > kThreshold$}{
    $J_{type} \gets revolute$
 }{
    $J_{type} \gets prismatic$ \\ 
    $J_{axis} \gets \Vec{a}$ \\
    $J_{position} \gets \texttt{center\_of\_part}(id_{moved})$
}

\If{$J_{type}$ is revolute}{
    $\hat{\mathcal{P}} \gets \texttt{find\_overlap\_points}(\mathcal{P}_t, \;\; \mathcal{P}_{t-1})$ \\
    $J_{axis} \gets \texttt{fit\_line}(\hat{\mathcal{P}})$ \\
    $J_{position} \gets \texttt{center}(\hat{\mathcal{P}})$
 }
\end{algorithm*}
